# Supplementary material for: Fragile Glasses Associated with a Dramatic Drop of Entropy under Supercooling
Source: arXiv:1909.03240 ancillary file (2020-12-21)
Supplement: Supplementary file 1 [file Fragility_supplementary.pdf]

# Supplementary Information for Fragile Glasses Associated with a Dramatic Drop of Entropy under Supercooling

## I. MODEL DETAILS: DIFFERENCES FROM PREVIOUS DEFINITION

We now provide further details of the DPLM adopted in this work, focusing on the differences of this variant with respect to that in Ref. [1]. A main feature in this work is to study a bicomponent form of the pair-interaction energy distribution  $g(V)$ , generalizing a simple uniform distribution used in Ref. [1]. This has been discussed in the main text. Here, we explain other differences.

**Particle-dependent interactions:** In this work, we consider a particle-dependent interaction  $V_{kl}$  between nearest neighboring (NN) particles, which depends only on the particle labels  $k$  and  $l$  (see Eq. (1) of the main text). This is a simplification from Ref. [1] which uses a site-particle-dependent interaction  $V_{ijkl}$  with additional explicit dependences on the sites  $i$  and  $j$  at which particles  $k$  and  $l$  are located. In Ref. [1], the explicit site dependence was introduced to model different frustration states at different sites. It was already shown analytically in Ref. [1] that the same exact equilibrium statistics hold for both  $V_{ijkl}$  and  $V_{kl}$  types of interactions. We have verified that adopting either  $V_{ijkl}$  or  $V_{kl}$  gives qualitatively similar features for all numerical measurements reported in Ref. [1] and in this work. Only minor quantitative differences are observed in general.

Although both  $V_{ijkl}$  and  $V_{kl}$  interaction types should in principle be applicable in this work, the computation for the case of  $V_{ijkl}$  is more intensive and is thus not adopted. Specifically, the whole set of  $V_{ijkl}$  requires a memory allocation of size  $\sim N^3 \sim L^6$ , for the case of  $N$  particles in a nearly fully occupied lattice of linear size  $L$ . Using a two-step interaction energy tabulation approximation, the requirement reduces to a manageable size of  $\sim N^2$ . This approximation has been verified to be accurate for  $G_0 = 1$  in particular by checking that the system energy  $E$  [see Eq. (1)] measured from simulations agrees with an exact theoretical value [1]. However, we find in this work that the accuracy can deteriorate as  $G_0$  decreases because the approximation admits strong finite size effects. For example, for  $G_0 = 0.01$ ,  $L = 100$  and  $T = 0.22$ , the measured  $E$  deviates by about 18% from the theoretical value. The error reduces if a larger  $L$  is used, but memory requirements may then be too demanding. In contrast, using  $V_{kl}$  for the same conditions, the discrepancy in  $E$  decreases to only about 0.6%. The memory consumption to store the whole set of  $V_{kl}$  is also of a manageable size of  $\sim N^2$  without needing the two-step interaction energy tabulation approximation.

**Metropolis algorithm:** We apply a Metropolis form of

the particle hopping rate  $w$  in Eq. (3) with a hopping energy barrier  $E_0 + \max\{\Delta E, 0\}$ , where  $\Delta E$  is the change of the system energy  $E$  induced by the hop attempt and  $E_0$  is an energy barrier offset. The energy barrier must be non-negative in all cases and this requires  $E_0 \geq 0$ . In Ref. [1], an activated-hopping form of the rate was used instead. A similar enforcement of the non-negativity of the energy barriers leads to a constraint  $E_0 \geq 1.5$  for an analogously defined offset  $E_0$ . Both the Metropolis and the activated hopping algorithms are widely used dynamics in simplified forms and both satisfy detailed balance. Nevertheless, an offset of  $E_0 = 0$  is only possible for the Metropolis algorithm and it corresponds to the case of a small average barrier or equivalently large barrier fluctuations. We have found in this work that this is the regime in which the most fragile glass can be obtained. In addition, dynamical pathways with the minimum possible barriers consistent with detailed balance in general exist according to potential energy landscape calculations on amorphous silica [2]. The Metropolis form is thus adopted to realize a wider range of fragilities. Interestingly, our results suggest that very fragile glasses have large fluctuations in the particle hopping energy barriers, which may be more consistent with the Metropolis function than the activated hopping function.

## II. DETAILED SIMULATION RESULTS

**Diffusion coefficient and Mean square displacement:** Figure S1 shows our kinetic Monte Carlo simulation results on the mean square displacement  $\text{MSD}(t)$  versus  $t$  for the example of a fragile glass at  $G_0 = 0.01$  and  $E_0 = 0$ . At each temperature  $T$ , we extract the diffusion coefficient  $D$  from  $D = (1/2d) (\text{MSD}/t)$  with  $d = 2$  at sufficiently large  $t$  in the diffusive regime. Specifically, we require that  $t$  is large enough to ensure that  $\text{MSD} > 1$  and  $\text{MSD} \propto t^\gamma$  with  $0.95 \leq \gamma \leq 1$ . For other values of  $G_0$ , the MSD is similarly measured and all results on  $D$  are shown in Fig. 1 in the main text.

As observed in Fig. 1, the dependence of  $D$  on  $G_0$  for any given  $T$  is nonmonotonic. This can be explained as follows. The energy  $E$  of the system equals the sum of all realized pair interactions  $V_{s_i s_j}$  [See Eq. (1)].  $D$  is smallest when particle hops involve the maximum fluctuations in  $V_{s_i s_j}$ . This is because excitations from the very stable states slow down the dynamics. Take  $T = 0.25$  as an example. When  $G_0$  is small, nearly all  $V_{s_i s_j}$  equal  $V_1 = 0.5$  and this results in a high  $D$  in Fig. 1. When  $G_0 = 1$ ,  $V_{s_i s_j}$  are distributed mainly in the range  $(V_0 + k_B T) \pm k_B T$  with  $V_0 = -0.5$  and  $k_B = 1$ , which is still a narrow range. This hence also leads to a relatively high  $D$ . In contrast,

for  $G_0 \sim 0.3$ ,  $V_{s_i s_j}$  jumps between  $(V_0 + k_B T)$  and  $V_1$ , as neither component of the interactions are negligible. This results in large fluctuations in the energies of the configurations related by particle hops and hence a small  $D$ . The precise minimized point of  $D$  depends also on entropic effects and thus on  $T$ .

From Fig. S1, we observe the emergence of a plateau characteristic of glasses as  $T$  decreases. The MSD for the example of a strong glass has been shown in Ref. [1]. Compared with a strong glass, results on the fragile glass in Fig. S1 exhibits a much more stretched-out plateau at low  $T$ . Despite the shallow plateaus in the MSD shown in Fig. S1 and in Ref. [1], our systems at low  $T$  is in fact deeply supercooled, by common measures in typical lattice or molecular dynamics (MD) simulations. Due to the lack of lattice vibrations, lattice simulations even in deeply supercooled regime always show shallow plateaus (see e.g. [3]). The MSD in Fig. S1 more precisely represents MSD of coarse-grained particle positions. It can be compared directly with the MSD based on the evolution of particle positions in inherent structures [4], which have been demonstrated computationally to possess a much shallower plateau than those with vibrations [5]. If one would add to the MSD the contribution of vibrations using some adiabatic approach, the plateau will be located around  $\text{MSD} \simeq 0.1$ , a typical value for particles of unit size. The plateau will then become much broader and more pronounced.

We have performed independent simulations for different values of  $T$  and  $G_0$  primarily for  $E_0 = 0$  as discussed above. Results for other values of  $E_0 > 0$  can be trivially obtained from those at  $E_0 = 0$  by rescaling time by a factor  $\exp(E_0/k_B T)$ , without performing further simulations. The diffusion coefficient  $D$  at  $E_0 > 0$  is simply obtained by multiplying the corresponding value of  $D$  for  $E_0 = 0$  by a factor  $\exp(-E_0/k_B T)$ . Note that we define  $T_g$  as  $T$  at which  $D = D_r \equiv 0.1$ , where the reference  $D_r$  remains a constant admitting no rescaling. As  $D$  is rescaled,  $T_g$  is varied and is recalculated from  $D = D_r$ . Results on  $D$  and  $T_g$  accordingly calculated for various  $E_0$  are applied in Fig. 2 in the main text.

**Temperature dependent void density:** Simulations in the main text are done with a fixed void density  $\phi_v = 0.01$  for simplicity, which is a small value more appropriate for glasses at low  $T$  with limited free volumes. In reality,  $\phi_v$  should increase as  $T$  increases. To model this phenomenon, we perform further simulations at  $G_0 = 0.1$  and  $E_0 = 0$  assuming a  $T$  dependent  $\phi_v$  given by

$$\phi_v(T) = \phi_v^\infty e^{-E_v/k_B T}, \quad (\text{S1})$$

where  $\phi_v^\infty$  denotes the void density at the high  $T$  limit and  $E_v$  is the free energy cost of void formation. We take  $\phi_v^\infty = 0.30$  and  $E_v = 0.75$ . At high  $T$ ,  $\phi_v \simeq \phi_v^\infty$  so that voids are abundant and particles can diffuse relatively freely as expected in non-glassy liquids. At low  $T$ , the model crosses over to the case with  $\phi_v = 0.01$ , noting

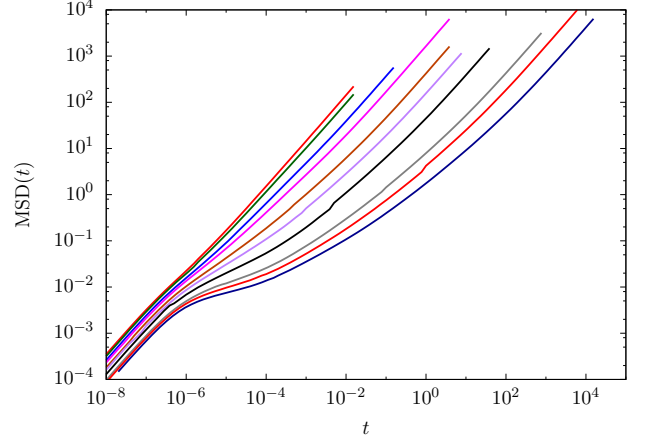

Figure S1.  $\text{MSD}(t)$  against  $t$  at  $G_0 = 0.01$  and  $E_0 = 0$ . Different curves represent different  $T = 0.4, 0.3, 0.24, 0.22, 0.2, 0.19, 0.18, 0.175, 0.17, 0.1667, 0.1626$  (from left to right).

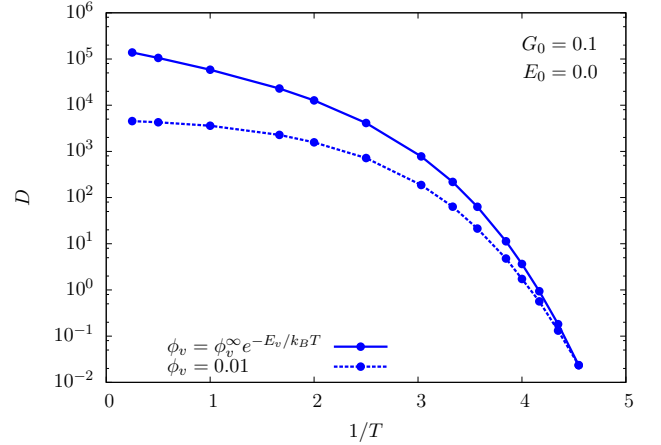

Figure S2. Arrhenius plot of  $D$  against  $1/T$  at  $G_0 = 0.1$  and  $E_0 = 0$  for a  $T$ -dependent void density  $\phi_v(T)$  and a constant  $\phi_v = 0.01$ .

$\phi_v(T = 0.22) = 0.01$ . The result on the diffusion coefficient  $D$  is shown in Fig. S2 and is compared with the case with a constant  $\phi_v = 0.01$ . Using  $\phi_v(T)$  from Eq. (S1),  $D$  becomes larger at high  $T$  due to the increased  $\phi_v$ . By defining  $T_g$  at  $D_r = 0.1$ , Fig. S3 plots  $D^{-1}$  against  $T_g/T$ . Also shown for comparison are examples of results for other values of  $G_0$  at  $\phi_v = 0.01$  from Fig. 2. We observe a spread of the high temperature limiting values of  $D^{-1}$  and this removes an artifact introduced by the constant  $\phi_v$  assumption. The fragility, which is predominantly a low  $T$  property, on the other hand is much less affected. For  $G_0 = 0.1$ , the kinetic fragility  $m_k$  computed using  $\phi_v(T)$  is 19.3. It is slightly higher than the value 16.2 found for the constant  $\phi_v = 0.01$  case. Therefore, results on fragility from our simple consideration of a constant  $\phi_v$  are expected to be valid in general.

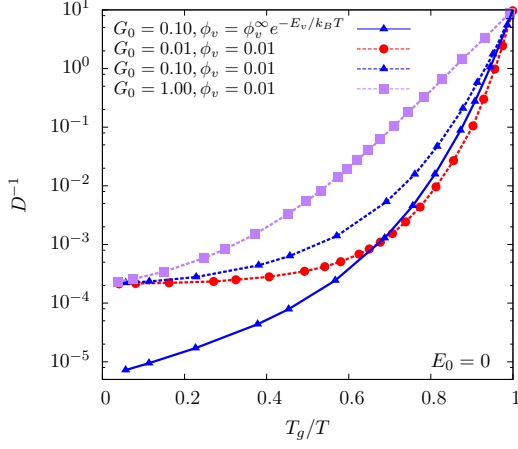

Figure S3. Kinetic Angell plot of  $D^{-1}$  against  $T_g/T$  for fixed void density  $\phi_v = 0.01$  at  $G_0 = 0.01, 0.1, 1$  and  $E_0 = 0$ , with the varying void density case at  $G_0 = 0.1$  and  $E_0 = 0$ .  $T_g$  is defined at  $D_r = 0.1$ .

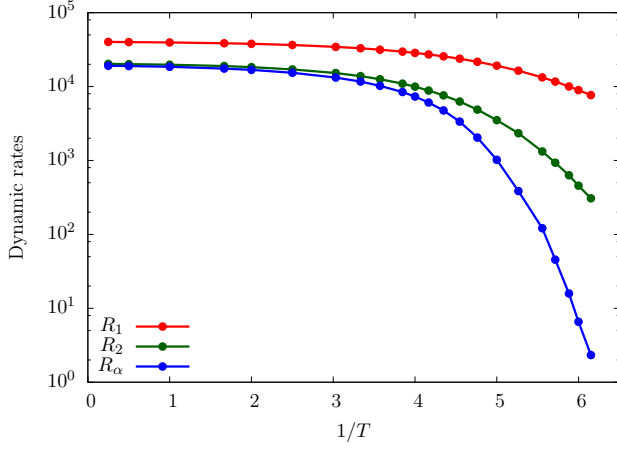

Figure S4. Rate of particle hops  $R_1$ , rate of particle non-returning second hops  $R_2$ , and structural relaxation rate based on mean square displacement  $R_\alpha$  against  $1/T$  at  $G_0 = 0.01$  and  $E_0 = 0$ .

**Hopping rates and return probability:** Glassy dynamics has strong temporal correlations characterized by numerous back-and-forth particle hopping motions. We now report analysis on dynamic rates and return probability to study the temporal correlations, following our previous works on polymer simulations [6, 7]. The hopping rate  $R_1$  of any individual particle is defined as the number of hops per particle per unit time. For our fragile glass with  $G_0 = 0.01$  and  $E_0 = 0$ ,  $R_1$  is measured from our simulations and results are reported in Fig. S4. For comparison, we have also plotted the structural relaxation rate  $R_\alpha = 1/\tau_\alpha$  where the relaxation time  $\tau_\alpha$  is extracted from the mean square displacement at MSD = 1 (see Fig. S1).

From Fig. S4, we see that  $R_1$  exhibits only a very mild super-Arrhenius slowdown compared with  $R_\alpha$  as  $T$

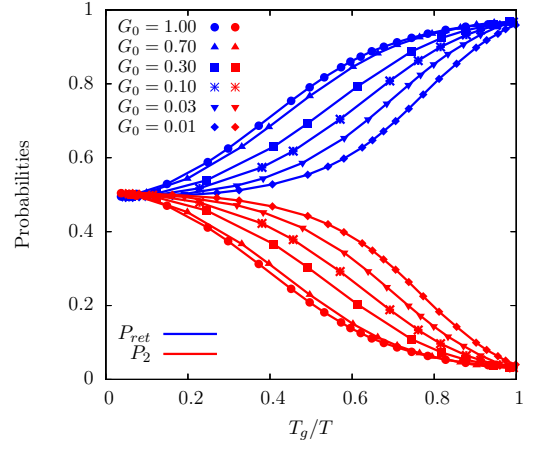

Figure S5. Probabilities of returning hop  $P_{ret}$  and non-returning second hop  $P_2$  against  $T_g/T$ , with  $T_g$  defined at  $D = D_r \equiv 0.1$ .

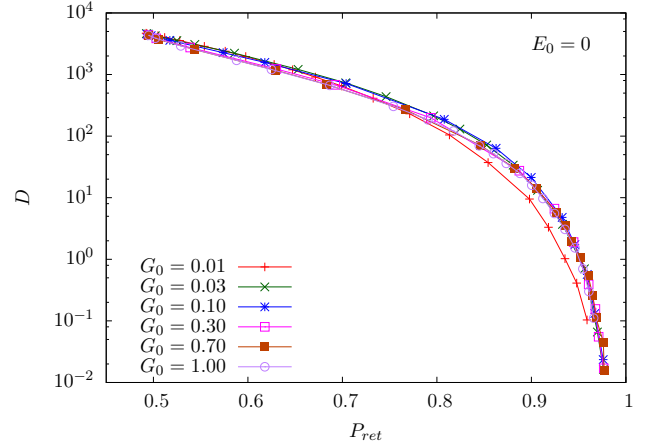

Figure S6. Plot of  $D$  against  $P_{ret}$  for various  $G_0$  and  $E_0 = 0$ .

decreases. Assuming isolated voids valid for the small  $\phi_v = 0.01$  used,  $R_1 = 4\phi_v \langle w \rangle$ , where  $\langle w \rangle$  is the average of the hopping rate  $w$  of a particle next to a void. As defined in Eq. (3),  $w$  depends on the hopping energy barrier  $E_0 + \Delta E$ , where  $\Delta E$  is the change of the system energy due to the hop. A mild  $T$  dependence of  $R_1$  thus implies a mild increase of the relevant hopping barriers as  $T$  decreases, which cannot explain the glassy slowdown.

To study hopping correlations, we monitor each particle after its first hop for a long duration. We measure the probability  $P_{ret}$  and  $P_2$  that it will next perform either a returning hop to its original position or a second hop to a third position respectively. The rate  $R_2 = P_2 R_1$  of a second non-returning hop is also shown in Fig. S4. It is clear that  $R_2$  exhibits a stronger super-Arrhenius  $T$  dependence than  $R_1$ . Compared with  $R_1$ , the value of  $R_2$  is closer to  $R_\alpha$  and can better characterize the glassy slowdown. Nevertheless,  $R_2$  still shows a slowdown milder than that of  $R_\alpha$ . This is because a sequence of two hops

to distinct positions is also often reversed and repeated at low  $T$  and may not characterize structural relaxations, as have been observed in polymer simulations [6]. It will be interesting to measure  $R_n$  with  $n \geq 3$  characterizing the rates of sequences of  $n$  non-returning hops after subsequences of back-and-forth hops in between are disregarded. Then,  $R_n$  at large  $n$  may show the same slowdown as  $R_\alpha$ .

Figure S5 plots  $P_{ret}$  and  $P_2$  against  $T_g/T$  for various values of  $G_0$ . Qualitatively, the result is very similar to that from polymer simulations in [6, 7]. In particular, it supports that  $P_{ret} \rightarrow 1$  when  $T \rightarrow 0$ .  $P_{ret}$  has reached 0.97 at the lowest  $T$  studied. A high  $P_{ret}$  clearly contributes to dynamic slowdown. It signifies highly constrained kinetic pathways resulting from a reduced entropy as argued in the main text. For the most fragile glasses at small  $G_0$ , we observe that  $P_{ret}$  rises with  $T_g/T$  most abruptly and the rise coincides with the abrupt drop of  $D$ . Furthermore, we plot  $D$  against  $P_{ret}$  for all  $G_0$  at  $E_0 = 0$  in Fig. S6, which shows a nice collapse of the data into a single curve. This further supports the strong relevance of  $P_{ret}$  to  $D$  and thus to  $m_k$ . Note that the collapse clearly breaks down for other values of  $E_0$  as only  $D$  but not  $P_{ret}$  depends on  $E_0$ . The properties of  $P_2$  is complementary to those of  $P_{ret}$  since  $P_{ret} + P_2 \simeq 1$ . The sum  $P_{ret} + P_2$  is slightly less than 1 because some particles do not perform a second hop even after a long duration.

**Self-intermediate scattering function:** Figure S7 shows the self-intermediate scattering function  $F_s(\mathbf{q}, t)$  [1] computed from our simulations for the fragile case at  $G_0 = 0.01$  and  $E_0 = 0$ , where  $\mathbf{q} = (2\pi/L)\mathbf{q}'$  with  $q' = 10$ . A very stretched-out relaxation is also observable at low  $T$ , analogous to results on the MSD. For example, the relaxation causing  $F_s(\mathbf{q}, t)$  to drop from 0.9 to 0.1 covers about three decades in time for the lowest  $T$  studied. Compared with results for a strong glass illustrated in Ref. [1], the decay in Fig. S7 for the fragile glass is significantly more stretched out.

Moreover,  $F_s(\mathbf{q}, t)$  in Fig. S7 shows apparently a single-step relaxation, which is indeed a two-step relaxation with a tiny first drop only noticeable upon magnification or in a semi-log scale, similar to the case of the strong glass in Ref. [1]. A small first relaxation step is again typical of lattice models due to the lack of vibrations. The main relaxation is well fitted by the Kohlrausch-Williams-Watts (KWW) stretched exponential function  $A \exp(-(t/\tau)^\beta)$  at sufficiently large  $t$  beyond the first relaxation step. Here,  $\beta$  is the stretching exponent while  $\tau$  and  $A \simeq 1$  are the relaxation time and the decay magnitude of the main relaxation. Specifically, we extract  $\beta$  from the fit around  $F_s(\mathbf{q}, t) = 1/e$ . For other values of  $G_0$ , values of  $\beta$  are similarly obtained.

Results for  $E_0 > 0$  can be obtained from those for  $E_0 = 0$  after performing a rescaling of time as explained above for the calculations of  $D$ . While the time rescaling alters  $F_s(\mathbf{q}, t)$ , it does not affect  $\beta$  for any fixed  $T$ . Therefore, the value of  $\beta$  at  $T_g$  depends on  $E_0$  only via  $T_g$ . Figure S8

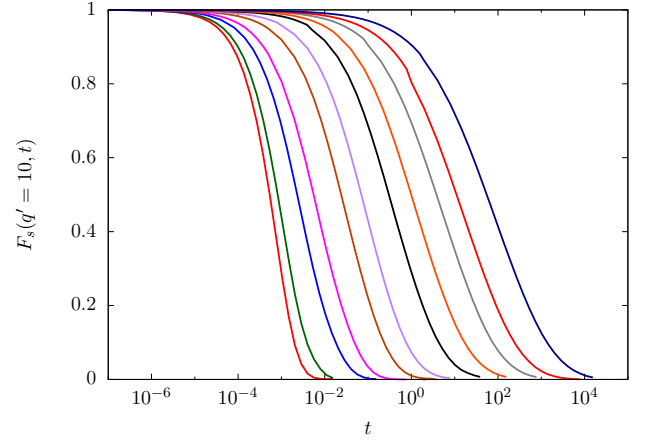

Figure S7.  $F_s(\mathbf{q}, t)$  against  $t$  at  $G_0 = 0.01$  and  $E_0 = 0$  with  $q' = 10$ . Different curves represent different temperatures at  $T = 0.4, 0.3, 0.24, 0.22, 0.2, 0.19, 0.18, 0.175, 0.17, 0.1667, 0.1626$  (from left to right).

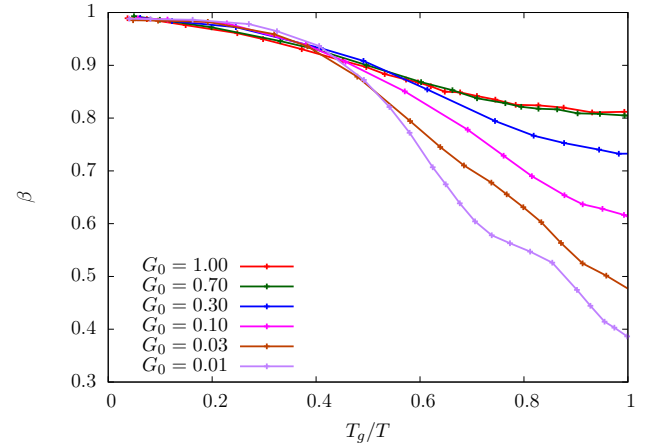

Figure S8.  $\beta$  against  $T_g/T$  at  $G_0 = 0.01, 0.03, 0.1, 0.3, 0.7, 1$ .  $T_g$  is extracted at  $D_r = 0.1$  for  $E_0 = 0$ .

shows the plot of  $\beta$  against  $T_g/T$  for all values of  $G_0$  at  $E_0 = 0$ . Using these and similar results for  $E_0 > 0$ , we perform third-order polynomial fits to the dependence of  $\beta$  on  $T_g/T$  to provide the best estimate of  $\beta$  at  $T_g$ , which are used in Fig. 3 in the main text.

We have also computed the structural relaxation time  $\tau$  defined using the self-intermediate scattering function by  $F_s(q' = 10, t = \tau) = e^{-1}$ . The corresponding Arrhenius plot and kinetic Angell plot are shown in Figs. S9 and S10, where  $T_g$  in Fig. S10 is defined as  $T$  at which  $\tau = 100$ . Qualitatively, results in Figs. S10 and 2 are fully analogous. Quantitatively, at low  $T$ ,  $\tau$  diverges faster than  $D^{-1}$ , leading to the Stoke-Einstein violation shown in Fig. S11. It is clear from Fig. S11 that the fragile systems exhibit a stronger violation.

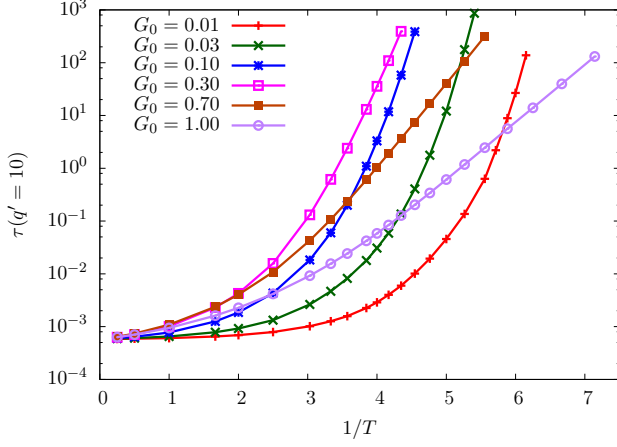

Figure S9. Arrhenius plot of  $\tau$  for various  $G_0$  at  $E_0 = 0$ .

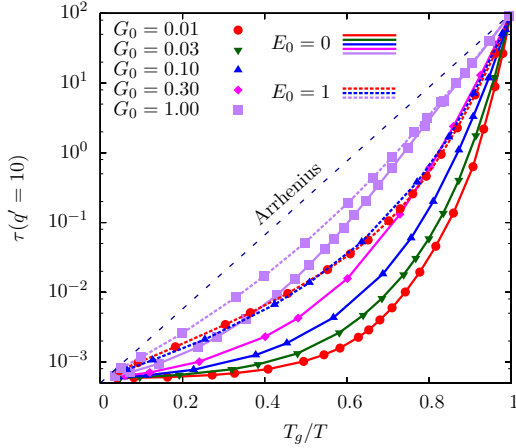

Figure S10. Kinetic Angell plot of  $\tau$  against  $T_g/T$  for various  $G_0$  and  $E_0$ , where  $T_g$  for each curve is defined at  $\tau_r = 100$ .

**Kinetic and thermodynamic fragilities:** We have calculated the kinetic and thermodynamic fragilities  $m_k$  and  $m_t$  for various values of  $G_0$  and  $E_0$ . Results are shown in Figs. S12 and S13 respectively. We observe empirically that for  $G_0 \lesssim 0.7$ , both  $m_k$  and  $m_t$  decrease linearly with  $\log G_0$ . Furthermore,  $m_k$  increases significantly as  $E_0$  decreases for small  $G_0$ . Otherwise, for  $m_t$  and  $m_k$  at large  $G_0$ , the dependence on  $E_0$  is weak. Combining the results in Figs. S12 and S13, we obtain the plot of  $m_t$  against  $m_k$  in Fig. 4 in the main text.

### III. KINETIC FRAGILITY EXTRAPOLATED TO REALISTIC TIME SCALE

Experimental values of the kinetic fragility  $m_k$  range typically from about 25 to 150 [8]. Our simulations give values from 6.76 to 26.35 which are in contrast a few times smaller. Nevertheless, this is only because we have adopted a large reference diffusion coefficient  $D_r = 0.1$  in

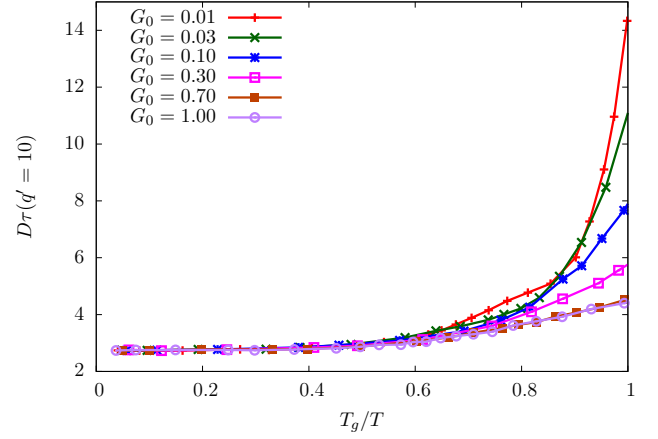

Figure S11. Plot of  $D\tau$  against  $T_g/T$  for various  $G_0$ , with  $\tau$  evaluated at  $q' = 10$  and  $T_g$  defined at  $D_r = 0.1$ . The non-constancy of  $D\tau$  with respect to  $T$  indicates the violation of the Stoke-Einstein relation.

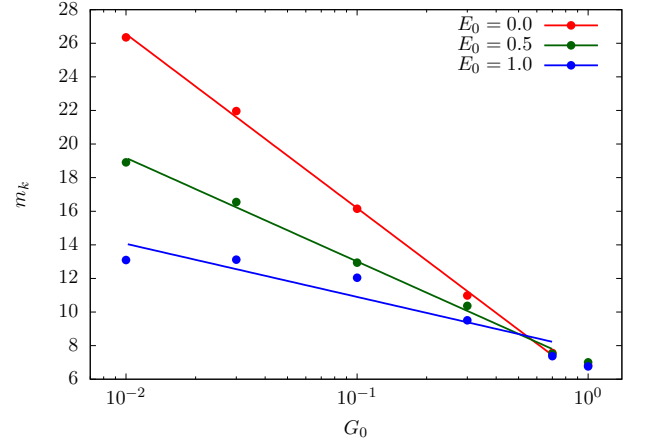

Figure S12.  $m_k$  against  $G_0$  at  $E_0 = 0, 0.5, 1$ .  $m_k$  is computed at  $D_r = 0.1$ .

the definition of  $T_g$  because of computational limitations. In fact, similar to all microscopic particle simulations, our DPLM simulations correspond to very short physical time scales compared with experimental situations. Adopting a much smaller  $D_r$  in direct analysis of simulations is not feasible because the required simulations would involve much slower dynamics. Here, we show that by extrapolating to a realistic value of  $D_r$ , corresponding to a much longer time scale, the obtained values of  $m_k$  increase significantly and are consistent with the typical experimental range.

We compute

$$m_k = \left. \frac{\partial \log D^{-1}}{\partial (T_g/T)} \right|_{T=T_g} \quad (\text{S2})$$

numerically from the values of  $D$  close to  $T_g$ . We define  $T_g$  as the temperature at which  $D = D_r$  with  $D_r = 0.1$ .

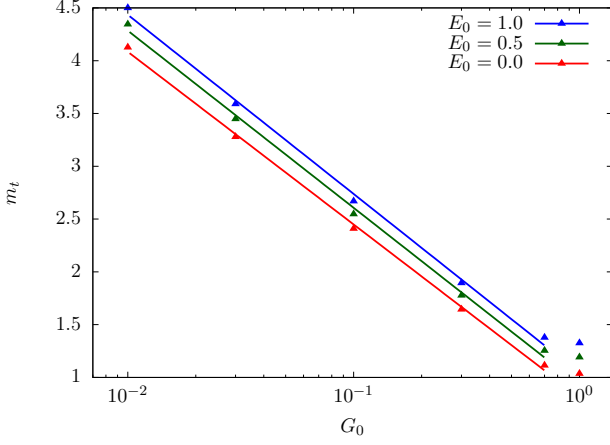

Figure S13.  $m_t$  against  $G_0$  at  $E_0 = 0, 0.5, 1$ .  $m_t$  is computed at  $T_g$  at which  $D_r = 0.1$ .

Let us first consider the strong glass limit corresponding to Arrhenius dynamics with the smallest possible kinetic fragility  $m_k^{strong}$ . As  $T \rightarrow \infty$ , the model reduces to a simple lattice gas. The diffusion coefficient is approximately given by

$$D_\infty \simeq \frac{(z-2)w_0\phi_v}{2d} \quad (S3)$$

with the coordination number  $z = 2d$  and dimension  $d = 2$  [9]. It evaluates to  $D_\infty \simeq 5 \times 10^3$  for small  $\phi_v = 0.01$ . Assuming an Arrhenius  $T$  dependence of  $D$ , Eq. (S2) gives  $m_k^{strong} = \log(D_\infty/D_r) \simeq 4.70$ . This is close to  $m_k = 6.76$  for the strongest glass we have considered at  $G_0 = 1$  and  $E_0 = 1$  in the main text. We next consider a more realistic value of  $D_r = 10^{-14}$ . This value is chosen so that as  $T$  varies from  $T_g$  to  $\infty$ ,  $D$  varies by nearly 18 orders of magnitude, a variation comparable to typical experimental ranges [10, 11]. This gives  $m_k^{strong} = 21.4$ , which is consistent with experimental values for strong glasses.

For the case of fragile glasses, we have obtained a large kinetic fragility  $m_k^{fragile} = 26.35$  at  $G_0 = 0.01$  and  $E_0 = 0$  based on  $D_r = 0.1$ . More generally, Fig. S14 plots  $m_k^{fragile}$  obtained from simulations for  $D_r = 0.2, 0.1414, 0.1, 0.707$  and  $0.05$ . For  $D_r < 0.1$ , we have performed a parabolic extrapolation to data in Fig. 1 and computed  $m_k^{fragile}$  using Eq. (S2) based on the extrapolated values of  $D$ . The result shows an empirical relation  $m_k^{fragile} \sim \ln D_r$ . An extrapolation using this relation to  $D_r = 10^{-14}$ , we get  $m_k^{fragile} = 120$ , which is more consistent with the experimental range. In principle, by extrapolating our simulation results towards  $G_0 \rightarrow 0$ , the kinetic fragility  $m_k$  appears to rise unboundedly.

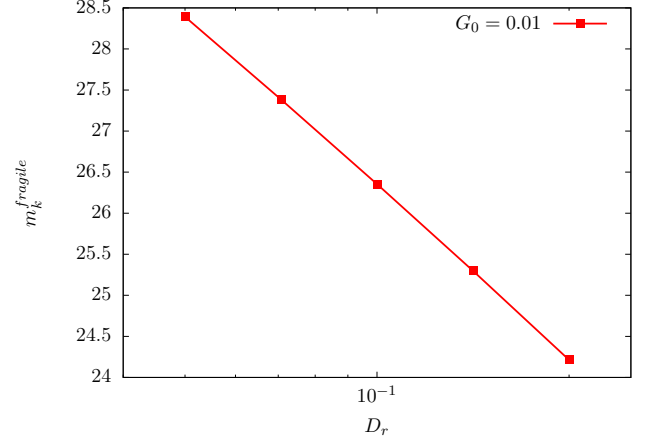

Figure S14. Kinetic fragility  $m_k^{fragile}$  against  $D_r$  for  $G_0 = 0.01$  and  $E_0 = 0$ .

#### IV. EXACT EQUILIBRIUM STATISTICS AND NUMERICAL VERIFICATIONS

We first summarize the equilibrium statistics of the DPLM on the 2D square lattice developed in [1]. Simulations are all performed in an canonical ensemble with a set of  $N$  particles. The partition function in canonical ensemble is given by

$$Z = \sum_{\{s_i\}} e^{-E/k_B T}, \quad (S4)$$

where the sum is over all possible particle configurations  $\{s_i\}$  and  $E$  is the system energy given in Eq. (1). Here,  $s_i$  denotes the particle at site  $i$ , with  $s_i = 0$  denoting instead a void. The occupation state at site  $i$  can be expressed as  $n_i = 1 - \delta_{s_i,0}$ , where  $\delta$  is the Kronecker delta. Equation (S4) can be rewritten as a sum over different occupation states as

$$Z = \sum_{\{n_i\}} Z_{\{n_i\}}, \quad (S5)$$

where the partition function for a given occupation state  $\{n_i\}$  is given by

$$Z_{\{n_i\}} = \sum_{\{s_i > 0\} \in \mathcal{P}_N} \prod_{<i,j>} e^{-V_{s_i s_j}/k_B T}. \quad (S6)$$

after using Eq. (1). Here,  $\mathcal{P}_N$  denotes the set of all permutations of the  $N$  particles and the product is over all nearest neighboring sites  $i$  and  $j$ .

At the thermodynamic (i.e. large  $N$ ) limit, it was shown in [1] that an average over particle permutations  $\mathcal{P}_N$  gives exactly

$$\frac{Z_{\{n_i\}}}{N!} = e^{-N_b U/k_B T}, \quad (S7)$$

where  $N_b$  is the number of nearest neighboring particle bonds in the system and  $U$  is the free energy of the corresponding interactions defined by

$$U = -k_B T \ln \int e^{-V/k_B T} g(V) dV. \quad (\text{S8})$$

Applying Eqs. (S5) and (S7), the exact partition function can be written as

$$Z = N! \sum_{\{n_i\}} e^{-N_b U/k_B T}. \quad (\text{S9})$$

Note that no ensemble averaging over the interactions  $V_{kl}$  has been performed yet, but they are already averaged out by the particle permutation averaging. Therefore, both quenched and annealed ensemble averaging over the interactions trivially arrive at the same exact partition function  $Z$  in Eq. (S9).

Using Eqs. (S5) and (S6) and the applicability of annealed averaging, it was shown in [1] that a realized interaction  $V_{s_i s_j}$  follows exactly the Boltzmann distribution

$$p_{eq}(V) = \frac{1}{\mathcal{N}} e^{-V/k_B T} g(V) \quad (\text{S10})$$

where

$$\mathcal{N} = \int e^{-V/k_B T} g(V) dV \quad (\text{S11})$$

is a normalization constant. The system energy  $E$  in Eq. (1) then gives

$$E = N_b^* \bar{V} \quad (\text{S12})$$

where  $N_b^*$  is the most probable value of the number of interactions in the system and  $\bar{V}$  is the average realized interaction energy given by

$$\bar{V} = \int V p_{eq}(V) dV. \quad (\text{S13})$$

The availability of an exact partition function  $Z$  in Eq. (S9) and the resulting exact equilibrium properties are remarkable properties of the DPLM. It is in our knowledge unique among energetically non-trivial models of glass defined on the square lattice and it has no counterpart for the closely related problem of spin glass. This highly surprising feature requires careful scrutiny. The exact distribution  $p_{eq}(V)$  in Eq. (S10) can be verified to a high precision by histograms of realized interactions in equilibrated systems. Examples of results are reported in [1] and [12]. The verification of the exact energy  $E$  in Eq. (S12) will also be explained later. Note that the validity of the exact expressions of  $p_{eq}(V)$  and  $E$  in Eqs. (S10) and (S12) rely directly on the validity of the exact partition function  $Z$  in Eq. (S9).

From Eq. (S9), it is clear that DPLM shares the same equilibrium particle occupation statistics with a simple lattice gas model with a uniform nearest neighboring particle interaction energy  $U$ . On the 2D square

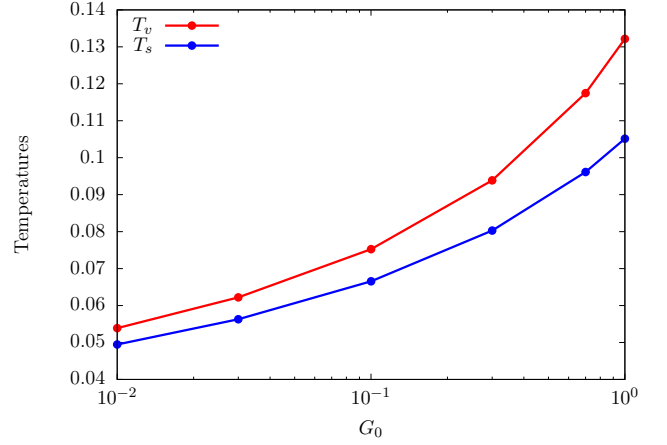

Figure S15. Vaporization temperature  $T_v$  and phase separation temperature  $T_s$  against  $G_0$ , where  $T_s$  is evaluated at a void density  $\phi_v = 0.01$ .

lattice, the simple lattice gas model admits a particle condensation-evaporation transition corresponding to the ferromagnetic-paramagnetic transition of the Ising model with an exchange interaction  $J = -U/4$  [13]. It occurs at a vaporization temperature  $T_v$ , given exactly by the Onsager solution [14]

$$T_v = \frac{-U}{2 \ln(1 + \sqrt{2})}. \quad (\text{S14})$$

For  $G_0 = 1$ , we get  $T_v = 0.132$  as evaluated in [1]. Figure S15 plots  $T_v$  for all values of  $G_0$ .

The condensation-evaporation transition at  $T_v$  is readily observable in the DPLM. We have observed from real-space animations at  $G_0 = 1$  and  $\phi_v = 0.5$  typical spinodal decomposition into co-existing particle and void aggregates as  $T$  is decreased below  $T_v$ . Theoretically, the exact partition function  $Z$  in Eq. (S9) remains valid both below and above  $T_v$  for the DPLM, analogous to the case of a simple lattice gas. The transition manifests itself through the non-analyticity of  $N_b^*$  and thus also of  $E$  at  $T_v$  [14].

In all simulations reported in this work, we consider  $T$  well above  $T_v$  so that no macroscopic void cluster exists. This is because in the evaporation phase, particle and void aggregates are miscible and two-phase co-existence is not applicable. It represents the physical regime we are interested in since large void aggregates do not typically exist in equilibrated supercooled liquids with few free volumes. Furthermore, large void aggregates in fact is not guaranteed to form even below  $T_v$  due to the small void density  $\phi_v$ . Below  $T_v$ , the occurrence of macroscopic aggregates of the minority component, i.e. the voids, is further controlled by the phase separation temperature  $T_s \leq T_v$ . Only for  $T < T_s$ , macroscopic particle condensates and void clusters become immiscible and phase separates. Here,  $T_s$  is obtained by solving the Onsager-Yang equation [15, 16]. For the DPLM, it is given exactly

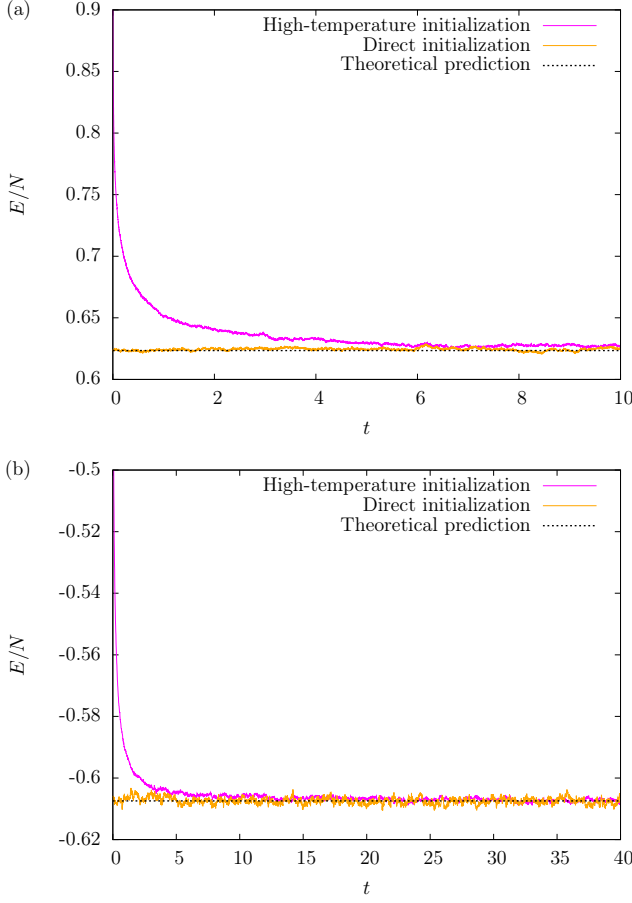

Figure S16. Plots of energy per particle  $E/N$  against time  $t$  from simulations at  $T = 0.2$  and  $\phi_v = 0.01$  using a high-temperature initialization (purple line) and a direct initialization method (orange line). The black dotted lines show theoretical predictions of the equilibrium values using Eq. (S18). We take  $G_0 = 0.01$  (a) and 1 (b).

by

$$T_s = \frac{-U}{2 \sinh^{-1} \left[ (1 - (2\phi_v - 1)^8)^{-\frac{1}{4}} \right]}. \quad (\text{S15})$$

For  $\phi_v = 0.01$ , the results on  $T_s$  for different  $G_0$  is also plotted in Fig. S15.

At a first sight, the possible occurrence of phase separation at  $T_v$  in addition to the glass transition at  $T_g$  appears to complicate the description of glass by the DPLM. However, this is not the case. From Eq. (S15), as  $\phi_v \rightarrow 0$ ,  $T_s \rightarrow 0$ , meaning that macroscopic void aggregates can be avoided at arbitrarily low  $T$  by selecting a sufficiently small  $\phi_v$ . There thus exists the physically relevant situation with an increasingly small void density  $\phi_v$  as  $T$  decreases (see e.g. Eq. (S1)) so that  $T_s$  is always below  $T$ . Thus, phase separation should not occur and no macroscopic void aggregate appears at any  $T$ .

Results above are exact for arbitrary  $\phi_v$ . Now, we assume a small  $\phi_v$  so that voids are mostly isolated. This is

justified for all simulations reported in this work because  $T \gg T_s$  with  $T_s$  shown in Fig. S15. Voids clusters must be so small that voids are isolated most of the time as is observable through the real-space visualizations (see Fig. 7 and videos in [1]). Assuming isolated voids, the number of particle interactions in the system follows

$$N_b = 2N(1 - \phi_v), \quad (\text{S16})$$

which is now a constant independent of the occupation state  $\{n_i\}$ . Using Eq. (S9), the partition function after summing over the occupation states is

$$Z = N! \mathcal{M} e^{-\beta N_b U}, \quad (\text{S17})$$

where  $\mathcal{M}$  is the number of possible particle occupation states. On the other hand, Eq. (S12) becomes

$$\frac{E}{N} = 2(1 - \phi_v) \bar{V}, \quad (\text{S18})$$

noting that  $N_b^* = N_b$ . The exact system energy  $E$  from Eq. (S18) is another non-trivial result following from the exact equilibrium statistics and the isolated void assumption. To verify its validity, Fig. S16 plots examples of the time-evolution of  $E/N$  for systems randomly initialized at  $T = \infty$ . It converges well to the exact value from Eq. (S18). This verifies Eq. (S18) which in turn verifies both the exact equilibrium statistics and the isolated void assumption.

In our main simulations, we apply a direct initialization method introduced in [1]. Specifically, a simple lattice gas with interaction  $U$  is first equilibrated, which is a very rapid procedure even at low  $T$ . Unrealized interactions  $V_{kl}$  are then sampled based on the *a priori* distribution  $g(V)$  while the realized interactions  $V_{s_i s_j}$  are instead sampled from the *a posteriori* distribution  $p_{eq}(V)$  given in Eq. (S10). The system energy  $E$ , also shown in Fig. S16, is already stable right after the sampling. This verifies the validity of the direct initialization method and hence again of the exact equilibrium statistics from which the method is derived.

## V. ENTROPY AT SMALL VOID DENSITY

For small  $\phi_v$ , using the partition function  $Z$  given in Eq. (S17), the system entropy  $S$  can be calculated straight-forwardly. From simple combinatorics,  $\mathcal{M} = C(L^2, N_v)$ , where  $N_v = L^2 \phi_v \simeq N \phi_v$  denotes the number of voids. Using  $\ln n! \simeq n \ln n - n$ , we get

$$\ln \mathcal{M} = N_v (\ln(L^2/N_v) + 1) = N_v (1 - \ln \phi_v). \quad (\text{S19})$$

Using Eqs. (S17) and (S19), the Helmholtz free energy  $F = -k_B T \ln Z$  equals

$$F = N_b U - k_B T N_v (1 - \ln \phi_v) - k_B T N (\ln N - 1). \quad (\text{S20})$$

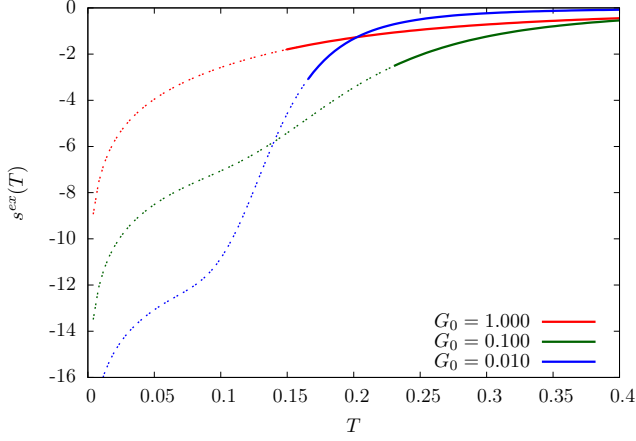

Figure S17. Equilibrium excess entropy per particle  $s^{ex}$  against  $T$  at various  $G_0$  for  $T > T_g$  (solid lines) and  $T < T_g$  (dotted lines). Note that results are of directly experimental relevance only for  $T > T_g$ , as equilibrium systems are in general available experimentally only under this condition.

From the thermodynamic relation  $F = E - TS$  with  $E = N_b \bar{V}$ , we get

$$S = \frac{N_b (\bar{V} - U)}{T} + N k_B \phi_v (1 - \ln \phi_v) + N k_B (\ln N - 1), \quad (\text{S21})$$

Defining the entropy per particle as  $s = S/N$ , we further define an excess entropy per particle  $s^{ex}(T) = s(T) - s^{LG}$  relative to the entropy  $s^{LG} = k_B \phi_v (1 - \ln \phi_v) + k_B (\ln N - 1)$  of a simple lattice gas [17]. Equations (S16) and (S21) then give

$$s^{ex} = \frac{2(1 - \phi_v)(\bar{V} - U)}{T} \quad (\text{S22})$$

Applying Eqs. (2), (S8), (S10) and (S13) and after some straight-forward algebra, we get

$$s^{ex} = 2k_B(1 - \phi_v) \left\{ 1 + \ln \left[ (G_0/\Delta V) k_B T (1 - e^{-\Delta V/k_B T}) + (1 - G_0) e^{-\Delta V/k_B T} \right] + \frac{[(1 - G_0)\Delta V/k_B T - 1]}{(G_0/\Delta V) k_B T (e^{\Delta V/k_B T} - 1) + (1 - G_0)} \right\}, \quad (\text{S23})$$

which is exact at the small  $\phi_v$  limit. Figure S17 shows the result for  $s^{ex}$  at  $G_0 = 0.001, 0.01, 0.1$ , and  $1$ . As  $T$  decreases, a significant drop of  $s^{ex}$  occurs around  $T \simeq 0.15$  and it becomes more and more dramatic as  $G_0$  decreases.

This dramatic and controllable drop of  $s^{ex}$  around  $T \simeq 0.15$  is the main cause of the high fragilities at small  $G_0$ . It results from a shift of the relative importance of the two components in  $g(V)$ . It can be intuitively understood by studying the interplay between the two components as follows. The bicomponent  $g(V)$  in Eq. (2) in the main text can be written as

$$g(V) = g_A(V) + g_B(V) \quad (\text{S24})$$

where components labeled  $A$  and  $B$  are the uniform and Dirac distributions given by

$$g_A(V) = \frac{G_0}{\Delta V}, \quad (\text{S25})$$

$$g_B(V) = (1 - G_0)\delta(V - V_1). \quad (\text{S26})$$

for  $V \in [V_0, V_1]$  with  $\Delta V = V_1 - V_0$ . Generalizing Eqs. (S11), (S13), (S8) and (S22) to individual components, we write

$$\mathcal{N}_{A,B} = \int e^{-V/k_B T} g_{A,B}(V) dV, \quad (\text{S27})$$

$$\bar{V}_{A,B} = \frac{1}{\mathcal{N}_{A,B}} \int V e^{-V/k_B T} g_{A,B}(V) dV, \quad (\text{S28})$$

$$U_{A,B} = -k_B T \ln \int e^{-V/k_B T} g_{A,B}(V) dV, \quad (\text{S29})$$

$$s_{A,B}^{ex} = \frac{2(1 - \phi_v)(\bar{V}_{A,B} - U_{A,B})}{T}. \quad (\text{S30})$$

which satisfy  $\mathcal{N} = \mathcal{N}_A + \mathcal{N}_B$ . These equations evaluate to

$$\mathcal{N}_A = \frac{G_0 k_B T}{\Delta V} e^{-V_0/k_B T} (1 - e^{-\Delta V/k_B T}), \quad (\text{S31})$$

$$\bar{V}_A = V_0 + k_B T - \frac{\Delta V}{e^{\Delta V/k_B T} - 1}, \quad (\text{S32})$$

$$U_A = V_0 - k_B T \ln \left[ \frac{G_0 k_B T}{\Delta V} (1 - e^{-\Delta V/k_B T}) \right], \quad (\text{S33})$$

$$s_A^{ex} = 2k_B(1 - \phi_v) \left\{ 1 + \ln \left[ \frac{G_0 k_B T}{\Delta V} (1 - e^{-\Delta V/k_B T}) \right] - \frac{\Delta V}{k_B T} \frac{1}{e^{\Delta V/k_B T} - 1} \right\}, \quad (\text{S34})$$

and

$$\mathcal{N}_B = (1 - G_0) e^{-(V_0 + \Delta V)/k_B T}, \quad (\text{S35})$$

$$\bar{V}_B = V_0 + \Delta V, \quad (\text{S36})$$

$$U_B = V_0 + \Delta V - k_B T \ln(1 - G_0), \quad (\text{S37})$$

$$s_B^{ex} = 2k_B(1 - \phi_v) \ln(1 - G_0). \quad (\text{S38})$$

Then,  $s^{ex}$  can alternatively be calculated using the standard expression for two-state systems:

$$s^{ex} = X s_A^{ex} + (1 - X) s_B^{ex} - X k_B \ln X - (1 - X) k_B \ln(1 - X), \quad (\text{S39})$$

where  $X = \mathcal{N}_A/\mathcal{N} = \mathcal{N}_A/(\mathcal{N}_A + \mathcal{N}_B)$  is the probabilistic weight of component  $A$ . Equation (S39) also evaluates to Eq. (S23) after some algebra. In Eq. (S39), the first two terms are the contributions of the two components alone. The remaining terms are the entropy due to the mixing of the components, which approaches 0 for  $X$  approaching 0 or 1.

Consider  $G_0 \ll 1$  corresponding to the regime relevant to fragile glasses. Eqs. (S31) and (S35) gives

$$\frac{\mathcal{N}_A}{\mathcal{N}_B} = \frac{G_0 k_B T}{\Delta V} e^{\Delta V/k_B T} (1 - e^{-\Delta V/k_B T}). \quad (\text{S40})$$

Then

$$\frac{\mathcal{N}_A}{\mathcal{N}_B} = \begin{cases} 0 & \text{for } T \rightarrow \infty \\ \infty & \text{for } T \rightarrow 0 \end{cases} \quad (\text{S41})$$

and hence

$$X = \begin{cases} 0 & \text{for } T \rightarrow \infty \\ 1 & \text{for } T \rightarrow 0. \end{cases} \quad (\text{S42})$$

Physically, component A corresponds to the low energy states important at low  $T$  while component B corresponds to the numerous states important at high  $T$ . Equation (S39) then implies

$$s^{ex} = \begin{cases} s_B^{ex}(T \rightarrow \infty) = 0 & \text{for } T \rightarrow \infty \\ s_A^{ex}(T \rightarrow 0) & \text{for } T \rightarrow 0 \end{cases} \quad (\text{S43})$$

where Eq. (S38) is also used. At  $T \rightarrow 0$ , Eq. (S34) simplifies to

$$s_A^{ex}(T \rightarrow 0) = 2k_B(1 - \phi_v) \left[ 1 + \ln \left( \frac{G_0 k_B T}{\Delta V} \right) \right], \quad (\text{S44})$$

and we have considered  $k_B T \ll \Delta V$  for simplicity. At small  $G_0$  and low  $T$ , due to the  $\ln G_0$  dependence,  $s_A^{ex}(T \rightarrow 0)$  is small and hence  $s^{ex}$  is also small. This explains the dramatic drop of  $s^{ex}$  from 0 as  $T$  decreases at small  $G_0$ .

## VI. BICOMPONENT INTERACTION DISTRIBUTION AND BOND EXCITATION MODEL

Note that the bicomponent  $g(V)$  in Eq. (2) is fully analogous to a bond excitation model, also called the two-state model, of glass proposed in Ref. [18], which considers microscopic states suggested as particle bonds taking either a low-entropy unexcited state or a high-entropy excited state. Although our component A is a band of

states, the energy spread becomes narrow at low  $T$  and this contributes to the similarity between the models. In Ref. [18], the entropy difference  $\Delta S^0$  and the enthalpy difference  $\Delta H^0$  between excited and unexcited state are the fitting parameters for the entropy for different materials. In our model, we can calculate  $\Delta S^0$  and  $\Delta H^0$  as follows. By dividing Eqs. (S34) and (S38) by  $2(1 - \phi_v)$ , we get the entropy per bond for the unexcited and excited state respectively. The entropy difference  $\Delta S^0$  is then  $\Delta S^0 = (s_B^{ex} - s_A^{ex})/[2(1 - \phi_v)]$ , which gives

$$\Delta S^0 = k_B \left\{ \ln \left[ \frac{(1 - G_0)}{G_0(1 - e^{-\Delta V/k_B T})} \frac{\Delta V}{k_B T} \right] + \frac{\Delta V}{k_B T} \frac{1}{e^{\Delta V/k_B T} - 1} - 1 \right\}. \quad (\text{S45})$$

On the other hand,  $\Delta H^0$  is simply given by  $\Delta H^0 = \bar{V}_B - \bar{V}_A$ . Using Eqs. (S32) and (S36),

$$\Delta H^0 = k_B T \left[ \frac{\Delta V}{k_B T} \left( 1 + \frac{1}{e^{\Delta V/k_B T} - 1} \right) - 1 \right]. \quad (\text{S46})$$

For the fragile glass with  $G_0 = 0.01$  and  $E_0 = 0$ , our DPLM simulations give  $T_g \simeq 0.163$ . Noting that  $k_B = \Delta V = 1$ , Eqs. (S45) and (S46) give  $\Delta S^0/k_B = 5.42$  and  $\Delta H^0/k_B T_g = 5.15$  at  $T = T_g$ . This can be compared with the fragile glass of toluene for example. By fitting to experimental results on entropy measurements, the bond excitation model gives  $\Delta S^0 = 45.4$  J/mol·K and  $\Delta H^0 = 6760$  J/mol, expressed in terms of per mole of excitable states [18]. Taking  $k_B = 8.315$  J/mol·K and  $T_g = 117$  K, they lead to  $\Delta S^0/k_B = 5.46$  and  $\Delta H^0/k_B T_g = 6.95$ . Toluene is considered because this value of  $\Delta S^0/k_B$  matches the value 5.42 from DPLM simulations. The consistency of the value of  $\Delta H^0/k_B T_g = 6.95$  with the DPLM result of 5.15 then provides an additional support of the close relation between the bond excitation model and the DPLM with the bicomponent form of  $g(V)$ .

- 
- [1] L.-H. Zhang and C.-H. Lam, “Emergent facilitation behavior in a distinguishable-particle lattice model of glass,” *Phys. Rev. B* **95**, 184202 (2017).
  - [2] T. Damart and D. Rodney, “Atomistic study of two-level systems in amorphous silica,” *Phys. Rev. B* (2018), 10.1103/PhysRevB.97.014201.
  - [3] W. Kob and H. C. Andersen, “Kinetic lattice-gas model of cage effects in high-density liquids and a test of mode-coupling theory of the ideal-glass transition,” *Phys. Rev. E* **48**, 4364 (1993).
  - [4] H.-Y. Deng, C.-S. Lee, M. Lulli, L.-H. Zhang, and C.-H. Lam, “Configuration-tree theoretical calculation of the mean-squared displacement of particles in glass formers,” *J. Stat. Mech.* **2019**, 094014 (2019).
  - [5] C. Y. Liao and S-H Chen, “Dynamics of inherent structure in supercooled liquids near kinetic glass transition,” *Phys. Rev. E* **64**, 031202 (2001).
  - [6] C.-H. Lam, “Repetition and pair-interaction of string-like hopping motions in glassy polymers,” *J. Chem. Phys.* **146**, 244906 (2017).
  - [7] C.-H. Lam, “Deeper penetration of surface effects on particle mobility than on hopping rate in glassy polymer films,” *J. Chem. Phys.* **149**, 164909 (2018).
  - [8] M. Matthieu, “Relaxation and physical aging in network glasses: a review,” *Rep. Prog. Phys.* **79**, 066504 (2016).
  - [9] C.-H. Lam, “Local random configuration-tree theory for string repetition and facilitated dynamics of glass,” *J. Stat. Mech.* **2018**, 023301 (2018).
  - [10] C. A. Angell, “Relaxation in liquids, polymers and plastic crystals — strong/fragile patterns and problems,” *J. Non-Cryst. Solids* **131-133**, 13 (1991).
  - [11] C. Alba, L. E. Busse, D. J. List, and C. A. Angell,

- “Thermodynamic aspects of the vitrification of toluene, and xylene isomers, and the fragility of liquid hydrocarbons,” *J. Chem. Phys.* **92**, 617 (1990).
- [12] M. Lulli, C. S. Lee, H. Y. Deng, C. T. Yip, and C. H. Lam, “Spatial Heterogeneities in Structural Temperature Cause Kovacs’ Expansion Gap Paradox in Aging of Glasses,” *Phys. Rev. Lett.* (2020), 10.1103/PhysRevLett.124.095501.
- [13] Andreas Nußbaumer, Johannes Zierenberg, Elmar Bitner, and Wolfhard Janke, “Numerical test of finite-size scaling predictions for the droplet condensation-evaporation transition,” *Journal of Physics: Conference Series* **759**, 012009 (2016).
- [14] M. Toda, R. Kubo, and N. Saito, *Statistical physics I: equilibrium statistical mechanics* (Springer, Heidelberg, 1991).
- [15] L. Onsager, “Statistical hydrodynamics,” *Il Nuovo Cimento Series 9* (1949), 10.1007/BF02780991.
- [16] C. N. Yang, “The spontaneous magnetization of a two-dimensional ising model,” *Phys. Rev.* **85**, 808 (1952).
- [17] J. C. Dyre, “Perspective: Excess-entropy scaling,” *J. Chem. Phys.* **149**, 210901 (2018).
- [18] C. T. Moynihan and C. A. Angell, “Bond lattice or excitation model analysis of the configurational entropy of molecular liquids,” *J. Non-Cryst. Solids* **274**, 131 (2000).
